# Supplementary material for: IE-Bench: Advancing the Measurement of Text-Driven Image Editing for Human Perception Alignment
Source: arXiv:2501.09927 source file (2025-01-17)
Supplement: Supplementary file 1 [file X_suppl.tex]

\clearpage
\setcounter{page}{1}
\maketitlesupplementary

\begin{figure*}[htp]
\centering
\includegraphics[width=1.7\columnwidth]{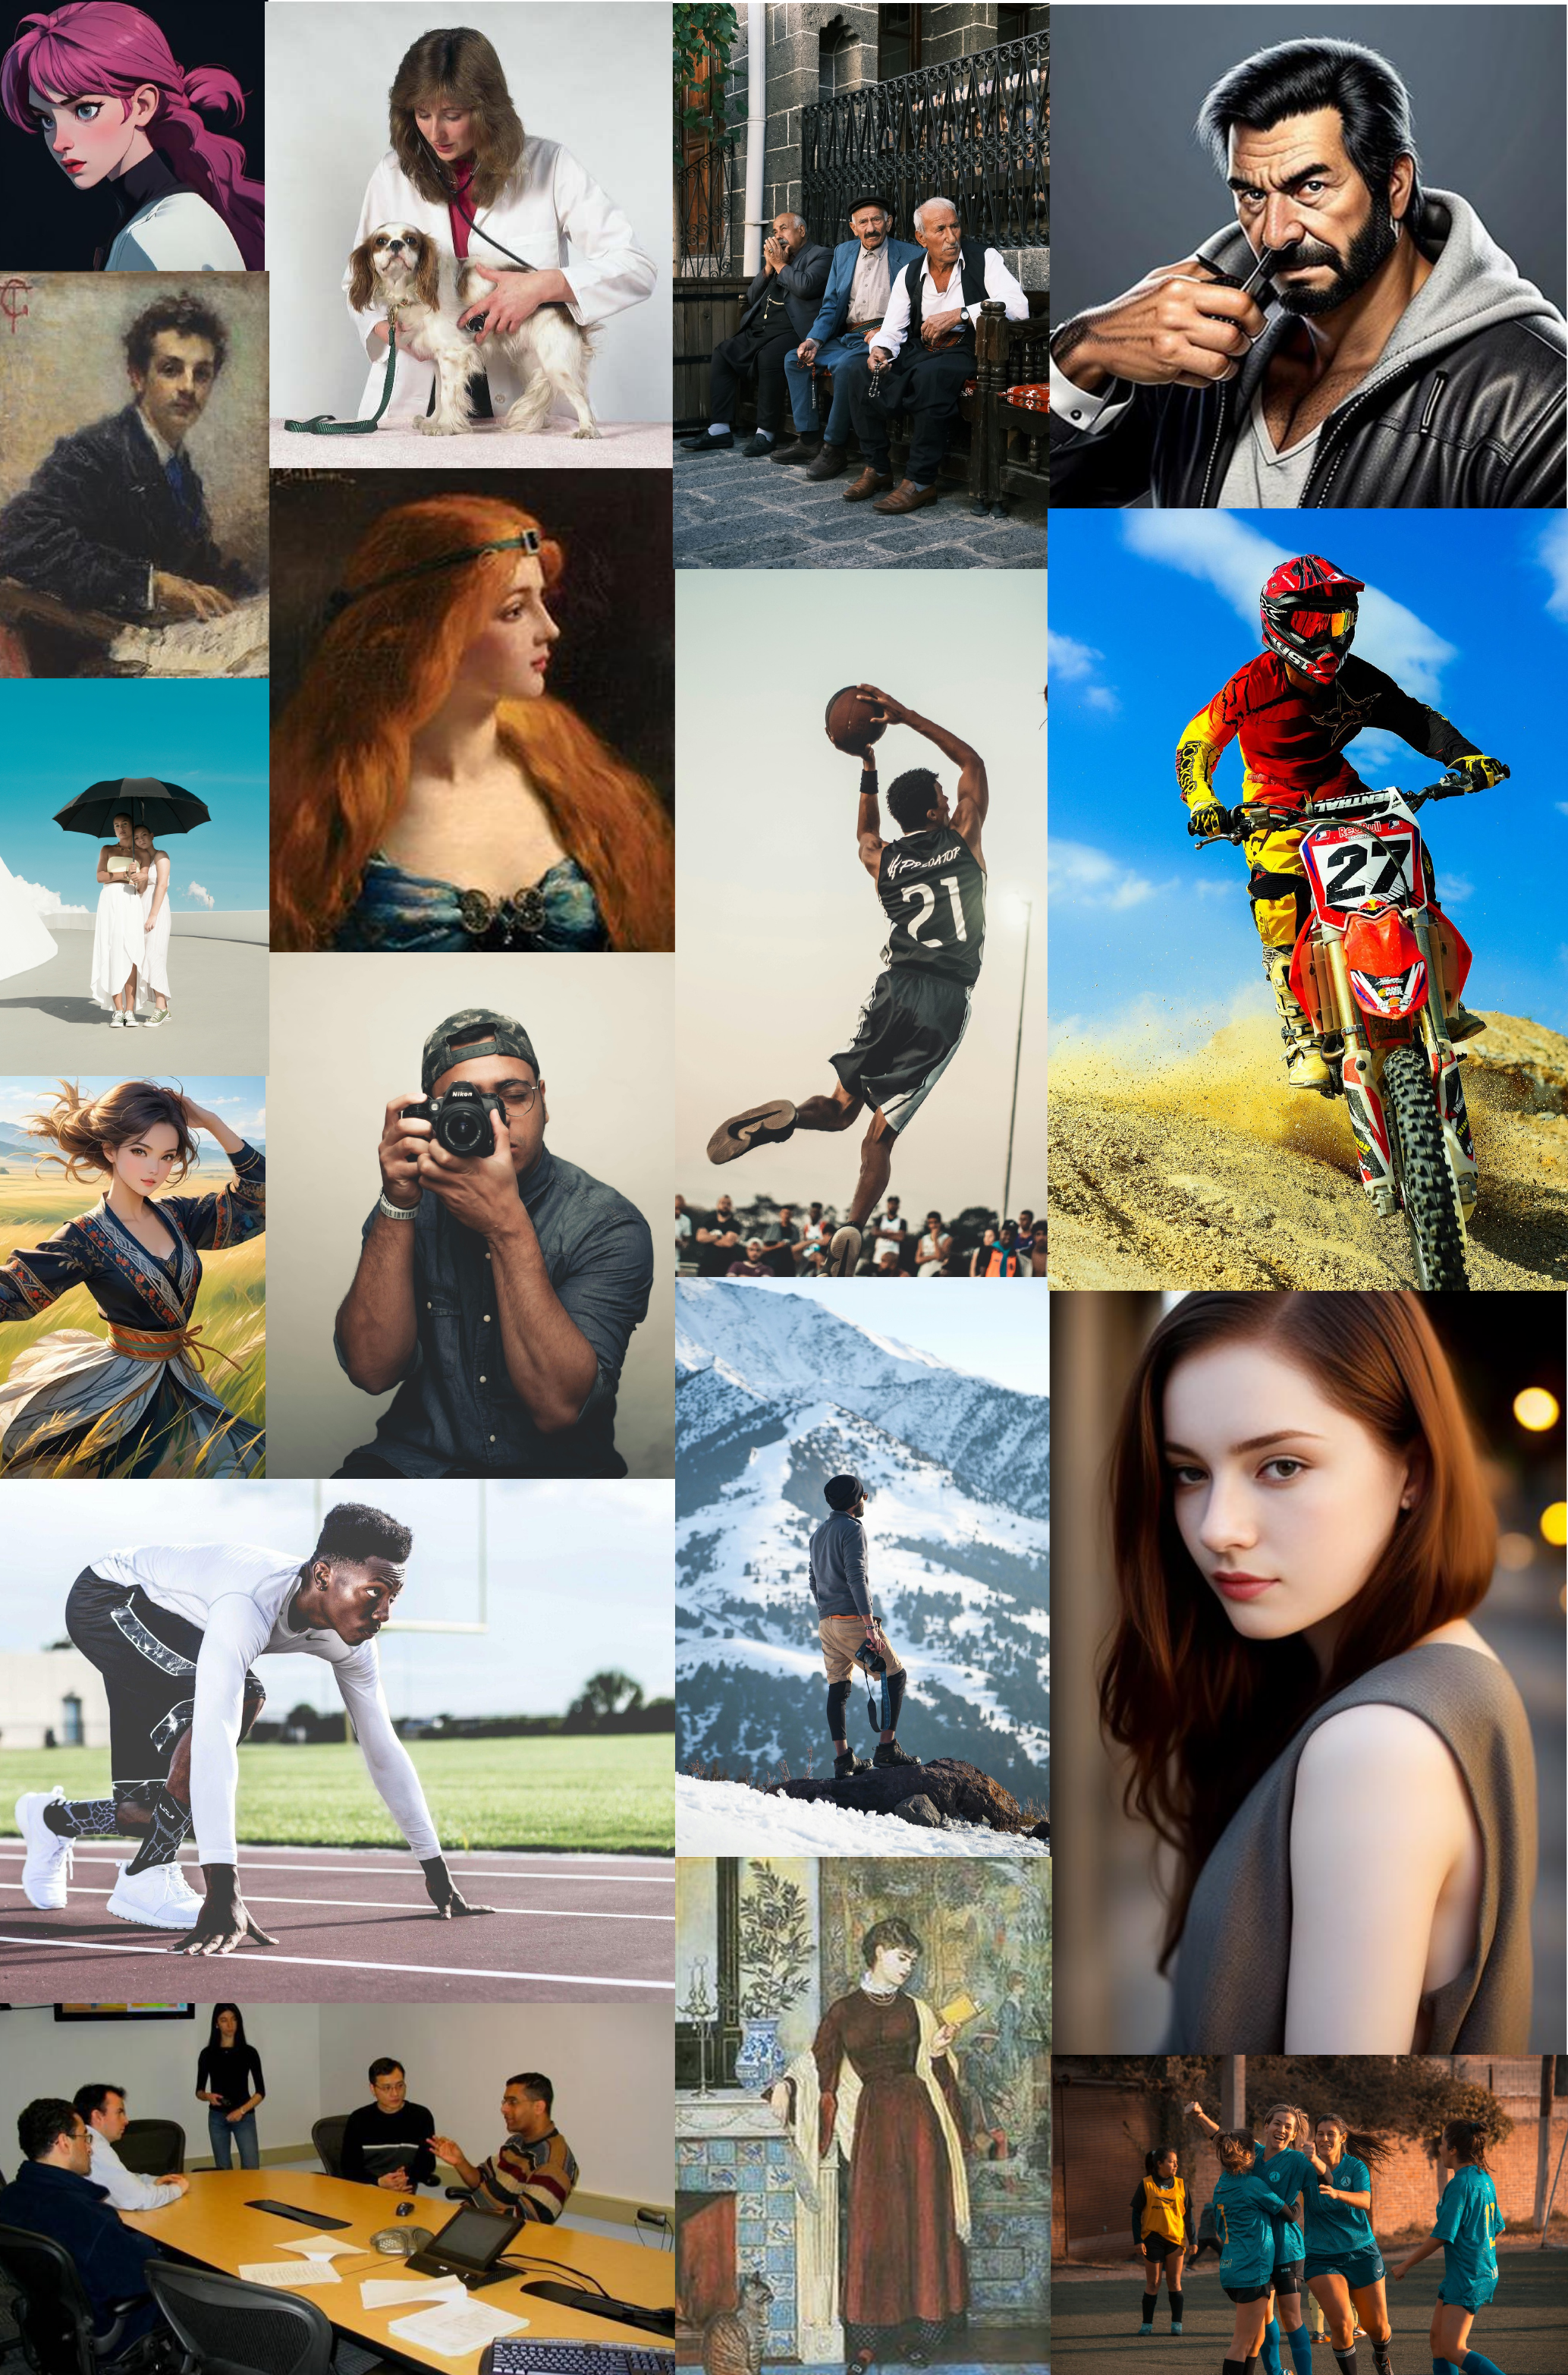} % Reduce the figure size so that it is slightly narrower than the column. Don't use precise values for figure width.This setup will avoid overfull boxes.
\caption{Examples in the collected human images.}
\label{fig:demo}
\end{figure*}

\section{Subjective Experiments}
All participants are over the age of 18, with at least an undergraduate education, coming from various backgrounds such as business, engineering, science, and law, and have independent judgment abilities. Following previous works~\cite{e-bench, t2iqa, t2vqa, keimel2012tum}, Prior to the experiment, all participants undergo offline training, during which examples of both good and bad edits, outside of the dataset, are shown. These examples are selected outside of the dataset to avoid introducing biases toward the cases in the dataset. Since the participants may not be familiar with the task at hand, the training lasts approximately one hour to ensure they fully understand the task. During the experiment, each participant rates all samples. Every 15 minutes of work is followed by a mandatory 5-minute break to prevent fatigue. The rating interface consists of three sections: the source image on the left, the edited result on the right, and two rows of text beneath the images. The first row displays the editing instructions, and the second row contains the corresponding rating options. The interface forces a 5-second stay on each sample, after which, once the participant submits their rating, the interface will move on to the next case.

\section{Source Image Collection}
When collecting data, we first confirmed that the data sources come from CG (computer-generated), AIGC (AI-generated content) images, artworks, real-world photos, etc., and identified relevant datasets. After confirming each dataset, we go through each sample, classify them according to different criteria, and apply appropriate labels. For example, images can be classified by content such as Nature, Object, Animal, Human, etc. The "Human" category is further subdivided based on the camera angle, such as half-body, full-body, and portrait, or by perspective (e.g., back view, side view, frontal view). Additionally, it can be categorized by factors like race, gender, or action type. We ensure a relatively balanced distribution through participant selection. We start by reviewing smaller datasets, prioritizing those with fewer samples, and then move on to larger datasets, selecting more diverse categories to supplement the collection. Finally, we supplement the dataset by gathering suitable content from the internet. This step is crucial. Although current datasets contain a rich variety of categories, most of the content still falls within conventional major categories. For example, landscape datasets typically include scenes like meadows or snowy mountains, but less common scenes like auroras, lava flows, and lightning are underrepresented. Additionally, despite the richness of current action classification datasets, there are still relatively few actions with large differences in pose or style.

Ultimately, our dataset contains over 100 different action categories for human subjects, including actions such as looking at the viewer, sitting, crossing arms, smiling, hand on hip, hand in pocket, holding a bag, raising one hand, looking forward, turning around, hands on head, twisting hands, looking at pictures, arms folded, talking, combing hair, sitting in a bathtub, playing karate, playing golf, holding a club, looking at a golf ball, dancing, thinking, crossing arms, raising hands, opening arms, blocking sunlight with hands, looking upward, looking at each other, playing with fireworks, holding a pigeon, opening mouth, pointing with a finger, attacking, raising a fist, squatting, holding a book, playing guitar, putting hands and feet on the floor, jumping, opening legs, bowing, hugging, holding arms out, putting hands on face, holding an umbrella, skateboarding, running, holding a ball, dragging, leaning, bending the body, shooting, taking pictures, closing eyes, riding, playing tennis, bending knees, throwing a ball, boating, doing yoga, drinking, climbing, squatting, putting hands on the floor, giving a high five, pushing up, hurdling, typing, playing basketball, playing soccer, kicking the ball, etc., as shown in the Figure~\ref{fig:demo}.

Sampling is also a good method for constructing datasets. One reason we did not sample from large-scale datasets is that the video resolution in large datasets, is often lower. Such samples contain limited detail and differ significantly from the viewing habits of the human eye, which can affect subjective experiments. In addition, to achieve an appropriate proportion across multiple classification dimensions and to collect as many action categories as possible, multiple rounds of sampling and manual screening are required. Therefore, this work ultimately chose to start with small datasets and manually screen samples, ensuring both efficiency and quality of the dataset.

% \section{Rationale}
% \label{sec:rationale}
% % 
% Having the supplementary compiled together with the main paper means that:
% % 
% \begin{itemize}
% \item The supplementary can back-reference sections of the main paper, for example, we can refer to \cref{sec:intro};
% \item The main paper can forward reference sub-sections within the supplementary explicitly (e.g. referring to a particular experiment); 
% \item When submitted to arXiv, the supplementary will already included at the end of the paper.
% \end{itemize}
% % 
% To split the supplementary pages from the main paper, you can use \href{https://support.apple.com/en-ca/guide/preview/prvw11793/mac#:~:text=Delete%20a%20page%20from%20a,or%20choose%20Edit%20%3E%20Delete).}{Preview (on macOS)}, \href{https://www.adobe.com/acrobat/how-to/delete-pages-from-pdf.html#:~:text=Choose%20%E2%80%9CTools%E2%80%9D%20%3E%20%E2%80%9COrganize,or%20pages%20from%20the%20file.}{Adobe Acrobat} (on all OSs), as well as \href{https://superuser.com/questions/517986/is-it-possible-to-delete-some-pages-of-a-pdf-document}{command line tools}.
